# Supplementary material for: Disentangled Human Body Embedding Based on Deep Hierarchical Neural Network
Source: arXiv:1905.05622 source file (2020-04-17)
Supplement: Supplementary file 1 [file supplement.tex]

\section{Supplement Explanation}
\edit{This is a supplementary description in supplement.tex about how to get the latent representations of a target mesh, need to be removed afterwards.}

\textbf{Latent Representation Extraction}. Given a mesh with our topology, we have two methods to get our latent representations. First, we use our encoder network to get latent representations. However, this method requires ACAP feature as input. As described in Gao~\cite{gao2017sparse}, to get ACAP feature, an integer optimization problem needs to be solved, which is time consuming for large human body mesh with complicated poses. Instead, we use the decoder part to get our latent representations reversely, which means we need to solve the point-to-point reconstruction problem,Sec~\ref{sec:pp_rec}:
\begin{equation}
    \min_{\mathbf{\beta},\mathbf{\theta}} \lambda\sum_i^{|\mathcal{V}|}\|\mathbf{p}_i(\mathbf{\beta},\mathbf{\theta})-\mathbf{q}_i\|+\lambda_{\beta}\|\mathbf{\beta}\|_2^2+\lambda_{\mathbf{\theta}}\|\theta\|_1
\end{equation}.
where $\mathbf{\beta}$ and $\mathbf{\theta}$ are shape and pose parameters separately and $\mathbf{p}_i(\mathbf{\beta},\mathbf{\theta})$ is $i_{th}$ point position of mesh decoded from $\mathbf{\beta},\mathbf{\theta}$, and $\mathbf{q}_i$ is the $i_{th}$ vertex of target mesh.

If the target mesh is not aligned with reference mesh orientation, we add rotation $\mathbf{R}$ and translation $\mathbf{T}$ to the optimization problem:
\begin{equation}
    \min_{\mathbf{\beta},\mathbf{\theta},\mathbf{R},\mathbf{T}} \lambda\sum_i^{|\mathcal{V}|}\|\mathbf{R}\mathbf{p}_i(\mathbf{\beta},\mathbf{\theta})+\mathbf{T}-\mathbf{q}_i\|+\lambda_{\beta}\|\mathbf{\beta}\|_2^2+\lambda_{\theta}\|\mathbf{\theta}\|_1
\end{equation}.
For this optimization with per point constraints, we assign $\lambda$ as $1.0\times6$, $\lambda_{\beta}$ and $\lambda_{\theta}$ as $1.0$. Our model generally takes about 300 iterators to achieve millimeter accuracy.

\textbf{Compare With PCA}.we also use PCA to embed our train data to latent representation. We train two version with PCA. For the first one we use whole train data to embed to a 128 dimensional latent representation. For the second one, we train two PCA models on shape and pose separately. We use our neutral shape data to train the shape model. As for pose PCA model, we use the 	difference of pose ACAP feature with corresponding neutral ACAP feature as the train data. Table~\ref{tab:test_recons} shows their reconstruction errors on the test dataset.

\begin{table}
\begin{center}
\begin{tabular}{|c|c|c|c|c|}
\hline
Test Dataset & ours & vae  & PCA(one)&PCA(two)\\
\hline\hline\hline
Neutral(159) & 6.2286 & 6.5997&6.0780 &7.6916 \\
Pose(80) & 3.9752 &6.0741 &10.2734 &17.0855 \\
\hline
\end{tabular}
\end{center}
\caption{point-to-point reconstruction error. Neutral pose test data has 159 meshes and pose test data has 80 meshes.}
\label{tab:test_recons}
\end{table}

\textbf{Dyna 300 Test Data Conversion Error}. point to plane error from smpl vertices without palm parts is about 2.7681mm with a std of 0.1617mm.

\textbf{Sparse Reconstruct Error}. We test our reconstruct error of sparse marker reconstruct with SMPL(remove some outlier results) and VAE. Table~\ref{tab:sparse_rec_39} and Table~\ref{tab:sparse_rec_22} show the results on 39 and 22 marker sets separately.

\begin{table}
\begin{center}
\begin{tabular}{|c|c|c|c|c|c|}
\hline
 & ours & smpl & vae \\
\hline\hline\hline\hline\hline\hline
all points & 13.4589 & 17.3198 & 16.8309\\
markers & 4.8792 & 12.4619 & 11.2413\\
\hline
\end{tabular}
\end{center}
\caption{Reconstruction error(mm) with 39 sparse markers constraints.}
\label{tab:sparse_rec_39}
\end{table}

\begin{table}
\begin{center}
\begin{tabular}{|c|c|c|c|c|c|}
\hline
 & ours & smpl & vae \\
\hline\hline\hline\hline\hline\hline
all points & 18.8953 & none & 19.5189\\
markers & 3.5163 & none & 11.0293\\
\hline
\end{tabular}
\end{center}
\caption{Reconstruction error(mm) with 22 sparse markers constraints.}
\label{tab:sparse_rec_22}
\end{table}

\textbf{Computing Time}. Our implementation is based on pytorch. The decoder from latent representation to mesh will take about 11ms on TITAN Xp GPU.

\textbf{Pose Parameter Replace}. We modify local pose parameters for our representation and SMPL separately. Fig.~\ref{fig:smpl_rep} shows an example. We modify the left elbows of first column meshes with middle column meshes, and third column are results. For SMPL, we just subtitute the pose parameters related to left elbow joint. The first row is SMPL's result, whose left hand moved into body, instead, our model generate more reasonable result.

\begin{figure}[t]
\begin{center}
\includegraphics[width=\linewidth]{images/smpl_replace.png}
\end{center}
   \caption{Examples of local pose subtitution of SMPL and ours. First row is SMPL result, which produce obviously self-intersection. Our model produce more reasonable result.}
\label{fig:smpl_rep}
\end{figure}
